# Supplementary material for: Depth Completion via Deep Basis Fitting
Source: arXiv:1912.10336 source file (2019-12-21)
Supplement: Supplementary file 1 [file appendix.tex]

\section*{APPENDIX}

Appendixes should appear before the acknowledgment.
